# Supplementary material for: Immersive and Interactive Visualization of 3D Spatio-Temporal Data using a Space Time Hypercube
Source: arXiv:2206.13213 source file (2022-06-27)
Supplement: Supplementary file 1 [file 5.1.additional.examples.tex]

%%commented on the main tex file

\section{Additional examples}\label{examples}

In this section, we present two additional examples of datasets\footnote{Details on the datasets can be found at https://morphonet.org/dataset under the names of ``Shoot-apical meristem'' and ``Sample 04''.}, also taken from the MorphoNet database, for which we generated STCs with the method previously described. 
The cutting plane capture resolution on these examples is 512x512. 
For each of the two datasets, we generated STCs based on three orthogonal cutting planes.

The first dataset shown in Figure~\ref{fig:examples}, left side, is a simulation in 42 time points of an abstract oryzalin-treated organ. The appearing outgrowth is obtained by locally softening the membrane of a shoot-apical meristem filled with uniform and steady turgor pressure. The stress magnitude on each cell, notably implied by this outgrowth, is colormapped on the STCs.
The second dataset, shown in Figure~\ref{fig:examples}, right side, is part of a 3D temporal imaging atlas of cell morphology for the C. elegans embryo. The recording includes 150 time points, from the 4 to 350 cells stages. The STCs displayed show the remaining lifespan of each cell as a colormap.

%\begin{figure}[t!]
%\centering
%\includegraphics[width=0.477\textwidth]{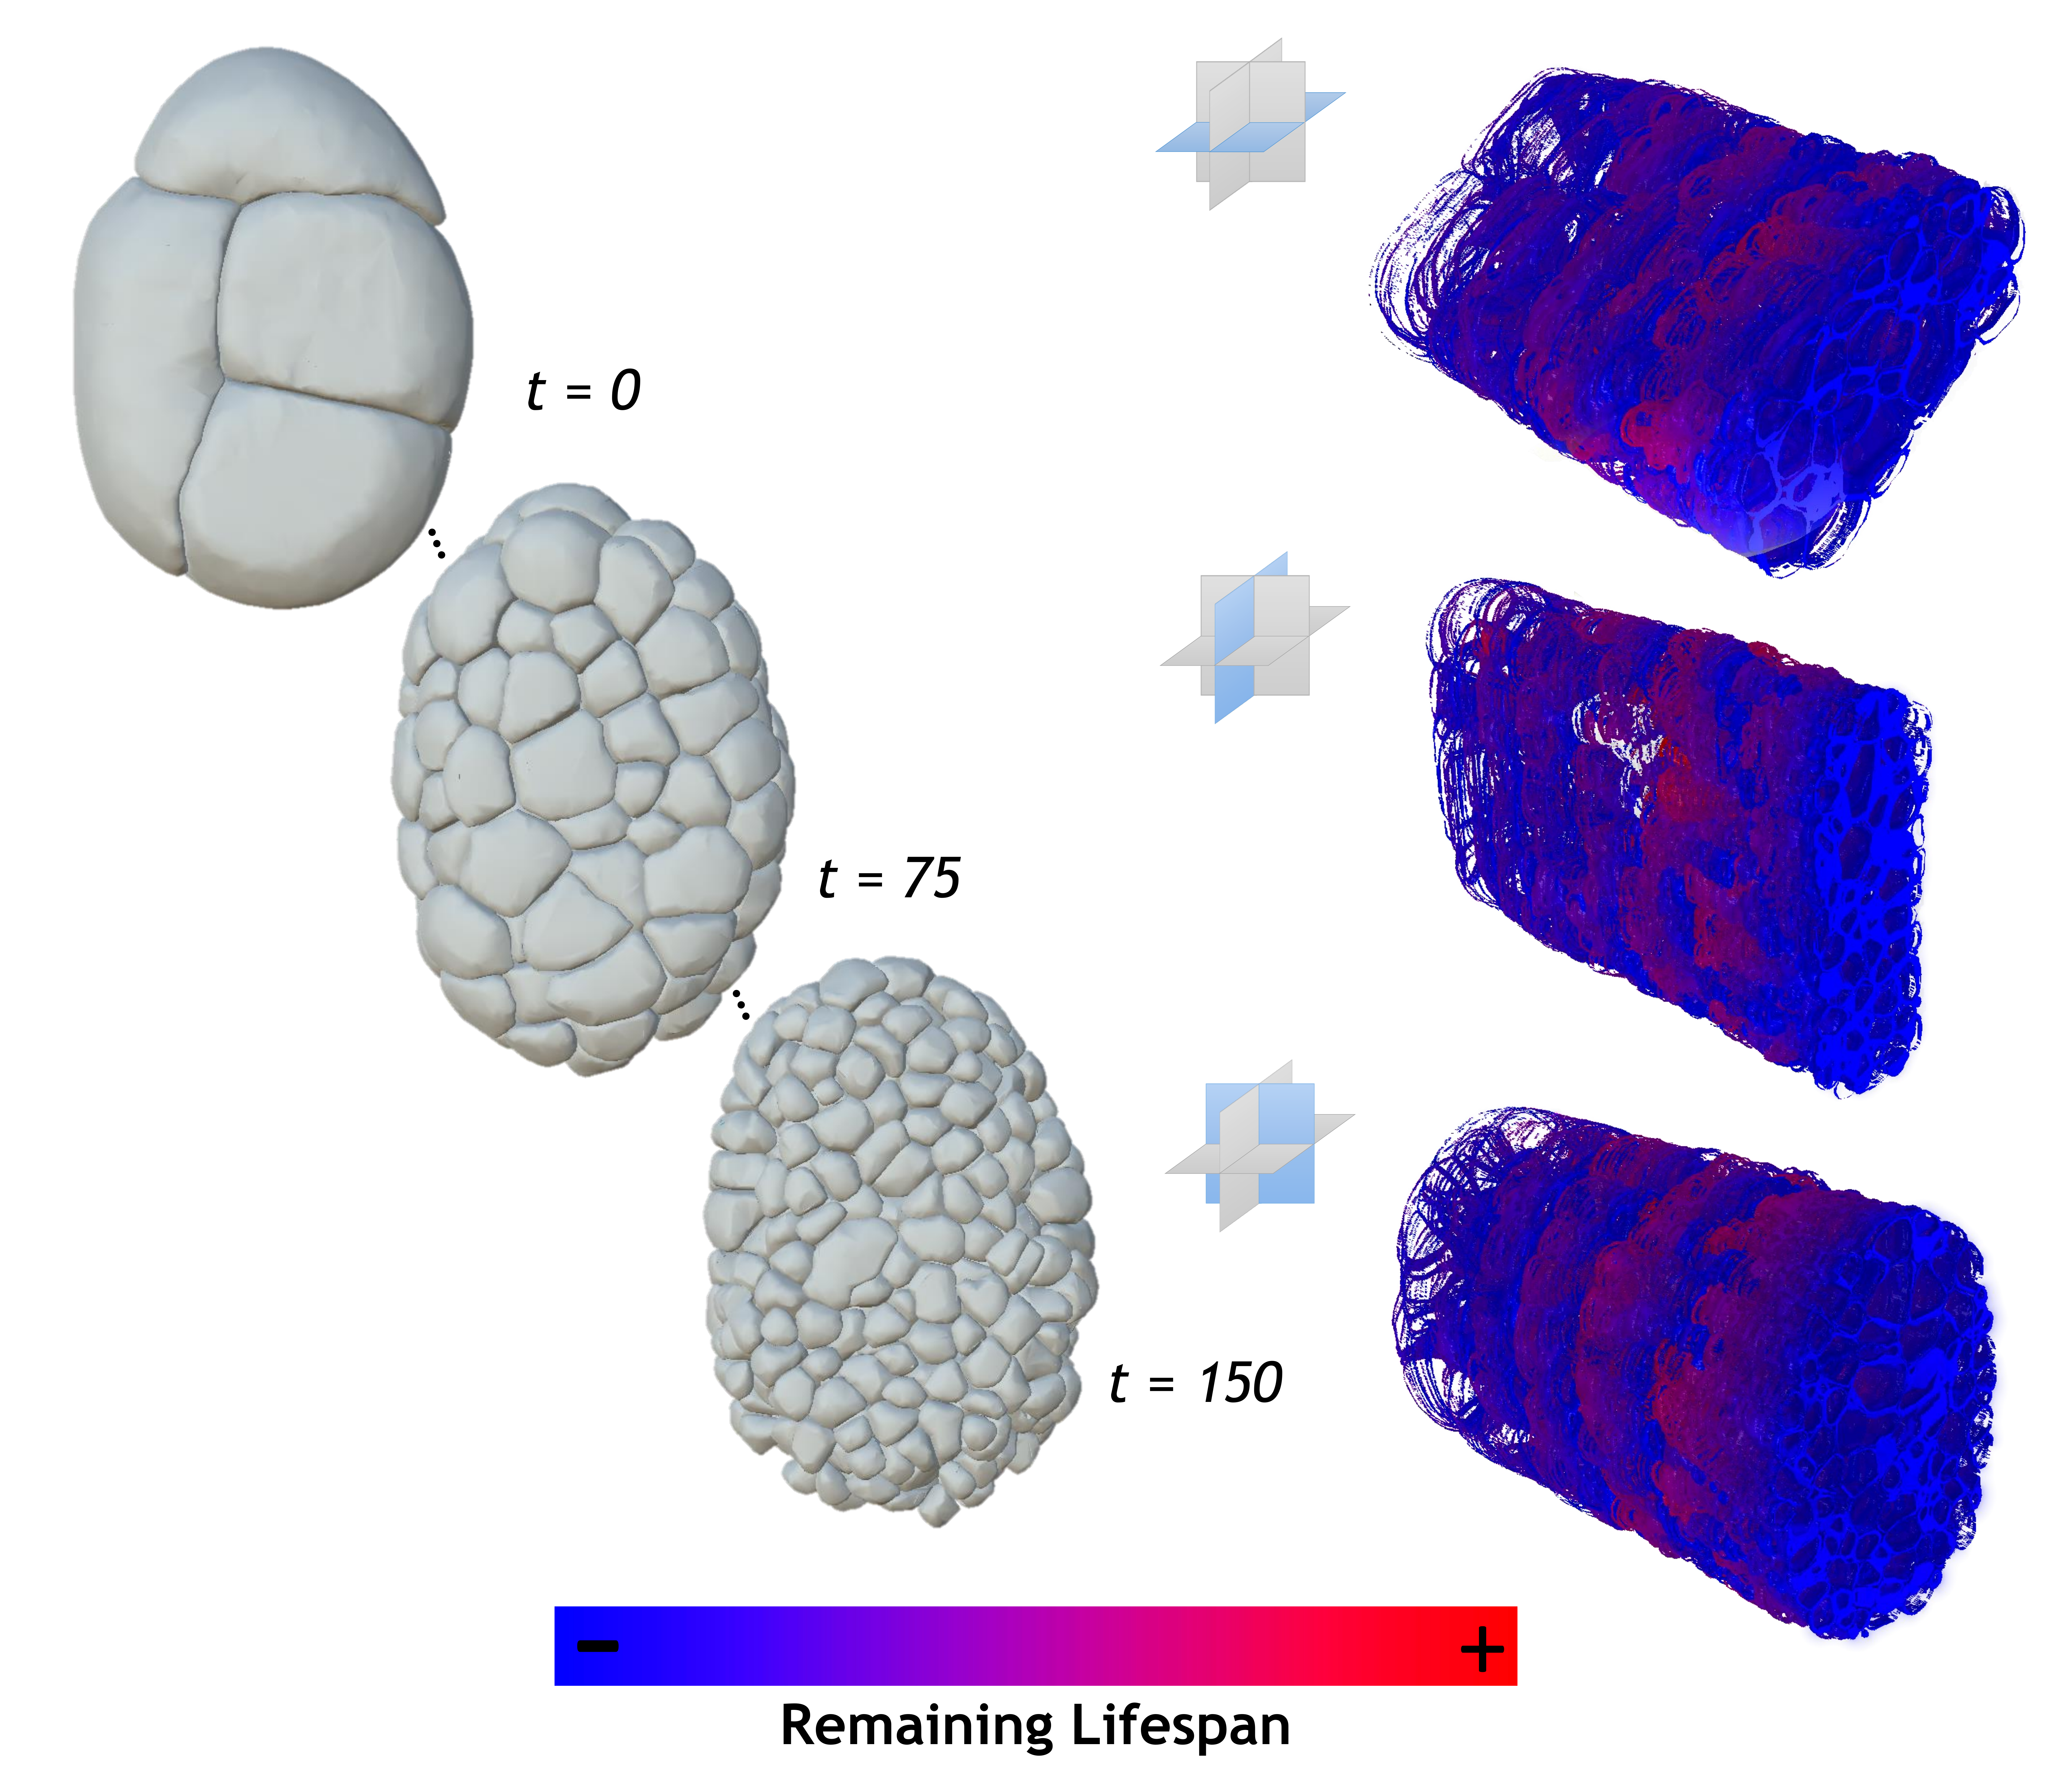}
%\caption{Examples of STCs with 3 different base planes for the capture, shown on the left pictures. The original dataset, from which 3 time points are displayed on the left pictures, is part of a 3D temporal atlas of the C. elegans embryo.}\label{fig:elegans}
%\end{figure} 
